# Supplementary material for: Exotic critical states as fractional Fermi seas in the one-dimensional Bose gas
Source: arXiv:2602.17656 source file (2026-06-10)

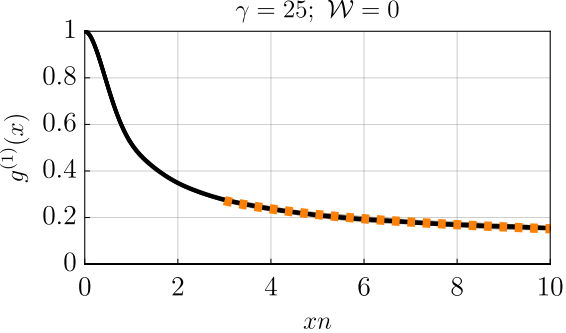

SD  
LD

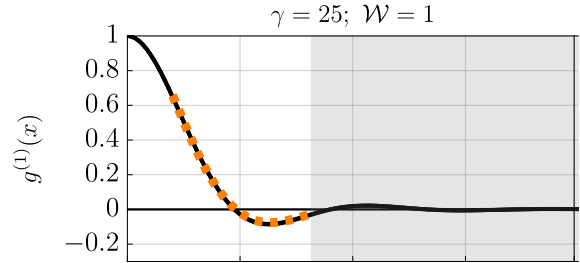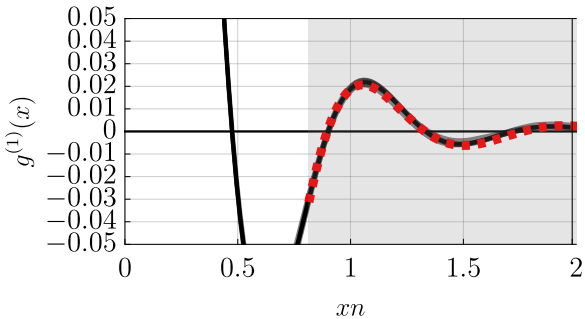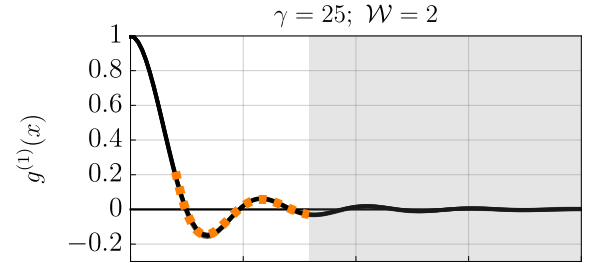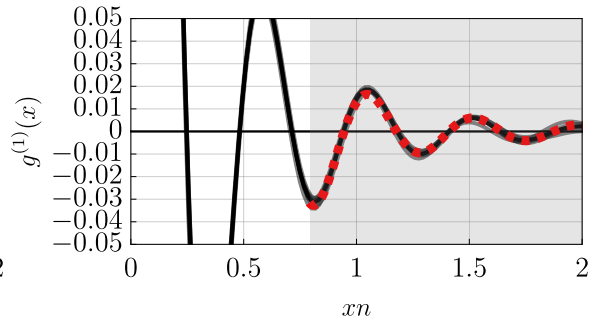

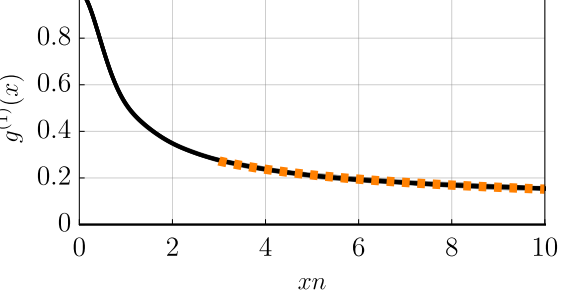

— SD  
— LD

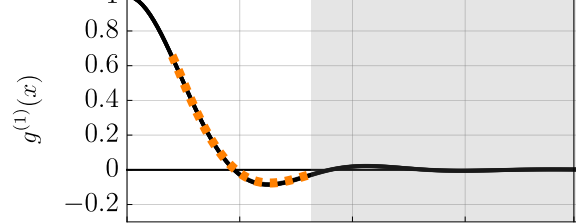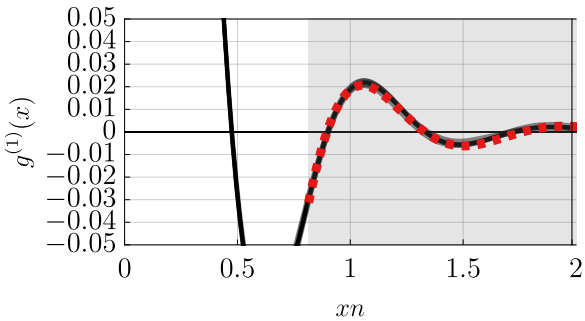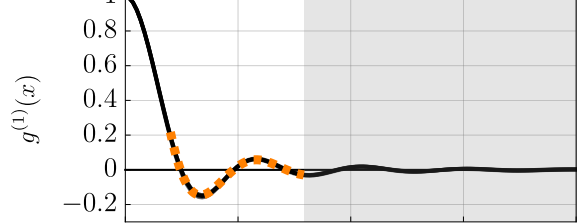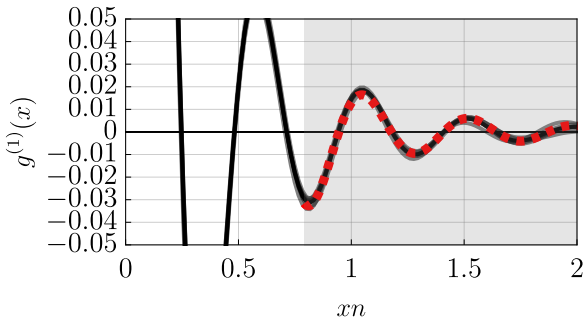

Supplement: Supplementary file 1 [file Fig_SM_Oscillations.pdf]
